# Supplementary material for: Query Circuits: Explaining How Language Models Answer User Prompts
Source: arXiv:2509.24808 source file (2026-06-01)
Supplement: Supplementary file 1 [file 6_use_of_large_language_models.tex]

\section{Disclosure of LLM Use}
\label{sup: use of large language models}
We utilize OpenAI ChatGPT, mainly GPT-5 and sometimes GPT-4o, to (1) aid and polish writing, and (2) retrieve and discover related literature. We manually verify all related works originally suggested by ChatGPT. None of the paragraphs are completely generated by ChatGPT.
