# Supplementary material for: Query Circuits: Explaining How Language Models Answer User Prompts
Source: arXiv:2509.24808 source file (2026-06-01)
Supplement: Supplementary file 2 [file feature_number_stats.tex]

\begin{table*}[tb]
\caption{\textbf{Number of gender-related SAE features under two different experimental settings.}
\textbf{Setting 1} compares independent groups of circuits partitioned by NDF using a one-sided Mann–Whitney U test.
\textbf{Setting 2} compares paired circuits constructed from the same samples (best vs.\ worst among 10 query circuits generated by paraphrases) using a one-sided Wilcoxon signed-rank test.}
\label{tab: gender-feature-stats}
\centering
% \small
\setlength{\tabcolsep}{8pt}

\resizebox{0.8\linewidth}{!}{
\begin{tabular}{@{}p{3.8cm} l c c c@{}}
\toprule
\textbf{Setting} & \textbf{Group} & \textbf{Mean $\pm$ Std} & \textbf{n} & \textbf{$p$-value} \\
\midrule
\multirow{2}{3.8cm}{\textbf{Unpaired Samples}} 
& $NDF > 0.8$ & $14.000 \pm 2.386$ & 27 & \multirow{2}{*}{0.3930} \\
\cmidrule{2-4}
& $NDF \leq 0.8$ & $13.609 \pm 3.327$ & 23 &  \\
\multicolumn{5}{l}{\quad $\Delta$ Mean = +0.391} \\
\midrule
\multirow{2}{3.8cm}{\textbf{Paired Samples}} 
& Best-among-10 & $14.625 \pm 2.733$ & \multirow{2}{*}{32} & \multirow{2}{*}{$< 0.0001$} \\
\cmidrule{2-3}
& Worst-among-10 & $19.906 \pm 4.122$ &  &  \\
\multicolumn{5}{l}{\quad $\Delta$ Mean = -5.281 \quad \textbf{(***)}} \\
\bottomrule
\end{tabular}}
\end{table*}
